# Supplementary material for: PSF-4D: A Progressive Sampling Framework for View Consistent 4D Editing
Source: arXiv:2503.11044 source file (2025-04-01)
Supplement: Supplementary file 1 [file X_suppl.tex]

% \clearpage
\setcounter{page}{1}
\maketitlesupplementary

\section{Overview}
\label{sec:overview}
The overview of the supplementary is as follows:
\begin{itemize}
    \item In Section~\ref{sec:preli}, we go over some of the preliminary knowledge required to better understand the diffusion process and 4D Gaussian Splatting. 
    \item In Section~\ref{sec:data_details}, we provide some details on the datasets used in the experiment.
    \item In Section~\ref{sec:training_details}, we present the details of training a 4D model and the steps to edit it.
    \item Section~\ref{sec:eval_metrics} describes the additional evaluation metrics used in this work.
    \item Section~\ref{sec:baseline_implement} contains the implementation details of previous SOTA methods.
    \item In Section~\ref{sec:quantitative_results}, we present a quantitative evaluation on different datasets as well as per-scene evaluation. 
    \item We describe the prompt design for local editing in Section~\ref{sec:local_editing}.
    \item Details of ablation study are provided in Section~\ref{sec:ablation_study}.
    \item We show a frame-by-frame comparison of PSF-4D and I4D-to-4D in Section~\ref{sec:comparison}.
    \item We provide a few edited 4D videos in a folder.
\end{itemize}
% We also address the minor typos\footnote{the reference for HyperNeRF dataset should be~\cite{park2021hypernerf}} here.

% \section{Why PSF-4D}

\section{Preliminaries}\label{sec:preli}
% \vspace{-1mm}
\paragraph{Gaussian Splatting (GS).} 3D Gaussian splitting (3DGS)~\cite{kerbl20233d} is a technique used in computer graphics and vision to represent complex 3D scenes by positioning Gaussian functions in space to approximate surfaces and volumes. In this method, each point in a 3D scene is represented by a Gaussian ellipsoid, defined by its center position \( \mathbf{p} \in \mathbb{R}^3 \), covariance \( \mathbf{\Sigma} \), and intensity \( I \). The Gaussian at each point \( \mathbf{p} \) is described by the function:
\begin{equation}
    G(\mathbf{x}) = I \, \exp\left(-\frac{1}{2} (\mathbf{x} - \mathbf{p})^\top \mathbf{\Sigma}^{-1} (\mathbf{x} - \mathbf{p})\right),
\end{equation}
where \( \mathbf{x} \in \mathbb{R}^3 \) represents a query point in space. By projecting these Gaussian onto a 2D image plane, a continuous, smooth approximation of the 3D scene is created, allowing for efficient rendering and visualization with realistic depth and detail. However, our work focuses on 4D Gaussian Splatting (4DGS)~\cite{yang2024deformable, wu20244d} model where 3DGS can be extended by incorporating per-frame dense tracking and novel view synthesis for dynamic scenes, leveraging a lightweight deformation field to represent Gaussian motions and shape variations across frames. 

\paragraph{Forward and Reverse Diffusion.} 
The diffusion phase spans a sequence of $T$ time steps. At each time step $t$, Gaussian noise is gradually added to the video latent $\boldsymbol{z}_0$ according to a defined variance schedule $\beta_1, \ldots, \beta_T$: 
\begin{align}
    q(z_{1:T}|z_0) &= \prod_{t=1}^{T}q(z_{t}|z_{t-1}), \\
    q(z_{t}|z_{t-1}) &= \mathcal{N} (z_{t}; \sqrt{1-\beta_{t}}z_{t-1},\beta_{t}\mathbf{I}).
\end{align}
With $\alpha_t={1-\beta_t}$ and $\overline{\alpha_t}=\prod_{s=1}^{t}\alpha_s$, the diffusion process can be expressed as: 

\begin{gather} 
q(z_{t}|z_{0}) = \mathcal{N} (z_{t}; \sqrt{\overline{\alpha}t}z_{0},(1-\overline{\alpha}_t)\mathbf{I}). 
\end{gather} 

Consequently, the noisy latent $z_t$ at each timestep $t$ can be sampled directly by: 
\begin{gather}
z_t = \sqrt{\overline{\alpha}_t} z_0 + \sqrt{1-\overline{\alpha}_t}\epsilon , \label{eq
} 
\end{gather} 
where $\epsilon \sim \mathcal{N}(\mathbf{0},\mathbf{I})$ represents Gaussian white noise matching the dimensions of $z_t$.

In the reverse denoising process using DDIM sampling, an image is generated by iteratively removing noise from an initially noisy latent representation. Starting from a latent \( z_T \) with maximum noise, the model predicts the clean latent for the next timestep \( z_{t-1} \) by leveraging a U-Net based noise estimator \( \epsilon_\theta \), which is trained to approximate the noise added during the forward diffusion. The update rule for each timestep \( t \) is defined as:
\[
z_{t-1} = \sqrt{\alpha_{t-1}} \left( \frac{z_t - \sqrt{1 - \alpha_t} \, \epsilon_\theta(z_t, t)}{\sqrt{\alpha_t}} \right) + \\ \sqrt{1 - \alpha_{t-1}} \, \epsilon_\theta(z_t, t),
\]
where \( \alpha_t \) and \( \alpha_{t-1} \) control the noise level at each step. This deterministic update allows DDIM to efficiently reach a high-quality output in fewer steps, providing a balance between image quality and generation speed.

\section{Experiment Details}

\subsection{Dataset Details}\label{sec:data_details}
\paragraph{DyNeRF Dataset.} utilized a mobile multiview capture system comprising 21 GoPro Hero 7 Black cameras, configured in linear mode at a resolution of $2704 \times 2028$ (2.7K) and a frame rate of 30 FPS. The cameras were synchronized using a timecode system, with intrinsic and extrinsic parameters calibrated through COLMAP~\cite{schonberger2016structure}. The dataset includes high-quality synchronized multi-view videos designed for 4D reconstruction of dynamic objects and view-dependent effects in natural indoor environments, addressing challenges not covered by existing public 4D datasets. As a pre-processing step, 60-second video sequences were split into chunks, alongside additional indoor and outdoor scenes with varying durations and keyframe densities. Eighteen camera views were used for creating the training set, with one reserved for evaluation, except for a multi-person sequence, which utilized 14 views. For our experiments, we extract 50 frame segments, from the full-length videos while rescaling the frames to a resolution of $1352 \times 1014$. 

\paragraph{HyperNeRF Dataset.} used a capture rig comprised of a pole with two Pixel 3 phones rigidly
attached roughly 16cm apart. This rig was used to collect a set of videos, each 30-60s long, sub-sampled to 15fps, and register the frames using COLMAP. The resolution is set to 960$\times$540. Some of the scenes we consider here are \emph{3D Printer, Chicken, Expressions, and Peel Banana}.

\paragraph{Dy-Check Dataset.} The Dy-Check dataset comprises 14 sequences showcasing non-repetitive motion across diverse categories, including generic objects, humans, and pets. The collection process utilizes three cameras: a hand-held moving camera for training purposes and two static cameras with a wide baseline for evaluation. A resolution of 480p is used for the experiment. 

\subsection{Training Details}\label{sec:training_details}
\paragraph{Original Model Initialization.} We follow the 4D Gaussian Splatting (4D-GS)~\cite{wu20244d} framework for building the initial 4D model and subsequent editing. 4D-GS extends 3D Gaussian Splatting to dynamic scenes by incorporating the temporal dimension, enabling efficient representation and rendering of spatial-temporal data. Instead of storing 3D Gaussians for each timestamp, 4D-GS maintains a single set of canonical 3D Gaussians and uses a Gaussian Deformation Field Network to model motions and deformations over time. This network comprises a lightweight and efficient spatial-temporal structure encoder, which consists of a multi-resolution HexPlane and a compact multi-head deformation decoder MLP. The HexPlane captures geometric and temporal relationships between adjacent Gaussians Instead of relying on the memory-intensive vanilla 4D neural voxel representation, we employ a 4D K-Planes module~\cite{kplanes} that decomposes the 4D neural voxel into six multi-resolution planes. Within this setup, all 3D Gaussians in a given region are encapsulated within the bounding plane voxels, while their deformations over time are efficiently encoded in the nearby temporal voxels.

% \begin{table*}[t]
% \centering
% \caption{ \textbf{Ablation Study} on different components of PSF-4D: \emph{auto-regressive noise model (ANM), cross-view noise model (CNM), and view consistent refinement (VCR)}.  We consider the DyNeRF dataset with 8 different prompts for this experiment.}
% % \vspace{-2mm}
% \label{tab:quantitative_comparison_ablation}
% \scalebox{0.8}{\begin{tabular}{l|ccccc}
% \toprule
% \textbf{Method} & \textbf{FID} $\downarrow$ & \textbf{CLIP Similarity} $\uparrow$ & \textbf{PSNR}$\uparrow$ & \textbf{SSIM}$\uparrow$ & \textbf{LPIPS}$\downarrow$ \\
% \midrule
% IN2N~\cite{haque2023instruct}+HexPlane~\cite{hexplane} & 64.27 & 0.2971 & 16.71 & 0.649 & 0.374 \\
% % Control4D~\cite{shao2023control4d} & 49.13 & 0.2980 & 17.60 & 0.658 & 0.388 \\
% I4D-to-4D~\cite{mou2024instruct} & 34.52 & 0.3068 & 19.92 & 0.706 & 0.419 \\
% \midrule
% PSF-4D \emph{w/o VCR} & 39.84 & 0.2941 & 17.36 & 0.673 & 0.397  \\
% PSF-4D \emph{w/o CNM} & 33.06 & 0.2994 & 19.84 & 0.692 & 0.418 \\
% PSF-4D \emph{w/o ANM} & 28.17 & 0.3078 & 20.96 & 0.714 & 0.427 \\
% PSF-4D & \textbf{22.58} & \textbf{0.3241} & \textbf{22.17} & \textbf{0.726} & \textbf{0.436}  \\
% \bottomrule
% \end{tabular}}
% % \vspace{-3mm}
% \end{table*}

\begin{table*} 
\centering
\small
\caption{\textbf{Quantitative results on all datasets}. For HyperNeRF, rendering resolutions are set to 960$\times$540 and 1352$\times$1014 for DyNeRF. On the other hand, we use a resolution of 480p for Dy-Check datasets. In total, 8 different prompts for each dataset is used in this experiment.}
\setlength{\tabcolsep}{13pt}
\scalebox{0.8}{\begin{tabular}{l|ccc|ccc|ccc} 
\toprule  
\textbf{Dataset} & \multicolumn{3}{c|}{\textbf{HyperNeRF}~\cite{park2021hypernerf}}  & \multicolumn{3}{c|}{\textbf{DyNeRF}~\cite{li2022neural}} & \multicolumn{3}{c}{\textbf{DyCheck}~\cite{gao2022monocular}} \\
\midrule
Model  &\textbf{PSNR}$\uparrow$ & \textbf{MS-SSIM}$\uparrow$ & \textbf{LPIPS}$\downarrow$ &\textbf{PSNR}$\uparrow$ &\textbf{SSIM}$\uparrow$& \textbf{LPIPS}$\downarrow$ &\textbf{PSNR}$\uparrow$↑ &\textbf{SSIM}$\uparrow$& \textbf{LPIPS}$\downarrow$ \\ 
\midrule  
IN2N~\cite{haque2023instruct}+HexPlane~\cite{hexplane}& 16.04 & 0.651 & 0.343  & 16.71 & 0.649 & 0.374 & 11.80 & 0.469 & 0.311 \\
% Control4D~\cite{shao2023control4d} & 16.82 & 0.681 & 0.360 & 17.60 & 0.658 & 0.384 & 12.76 & 0.488 & 0.327 \\
I4D-to-4D~\cite{mou2024instruct}& 19.65 & 0.736 & 0.371 & 19.92 & 0.706 & 0.419 &  14.10 & 0.516 & 0.337 \\
PSF-4D (Ours)& \textbf{21.48} & \textbf{0.781} & \textbf{0.395} & \textbf{22.17} & \textbf{0.726} & \textbf{0.436} &  \textbf{15.28} & \textbf{0.531} & \textbf{0.352} \\
\bottomrule
\end{tabular} }
\label{tab:comparison_all_datasets}
\end{table*}

\begin{table*}
\centering  
% \fontsize{6.5}{8}\selectfont  
\caption{Per-Scene results of DyNeRF's~\cite{li2022neural} datasets.} 
\label{tab:dynerf_comparison}  
\scalebox{0.9}{\begin{tabular}{l|cc|cc|cc}  
    \toprule  
    \multirow{2}{*}{\textbf{Method}}&  
    \multicolumn{2}{c}{\textbf{Cut Beef}}&\multicolumn{2}{c}{\textbf{Cook Spinach}}&\multicolumn{2}{c}{\textbf{Sear Steak}}\cr  
    \cmidrule(lr){2-3}\cmidrule(lr){4-5}\cmidrule(lr){6-7}
    &\textbf{PSNR}$\uparrow$&\textbf{SSIM}$\uparrow$&\textbf{PSNR}$\uparrow$&\textbf{SSIM}$\uparrow$&\textbf{PSNR}$\uparrow$&\textbf{SSIM}$\uparrow$\cr  
    \midrule  IN2N~\cite{haque2023instruct}+HexPlane~\cite{hexplane}&19.42&0.674&18.94&0.668&18.02&0.661\cr
    I4D-to-4D~\cite{mou2024instruct}&21.40&0.727&20.85&0.728&20.51&0.716\cr
    Ours&23.47&0.743&23.16&0.732&22.83&0.729\cr
\toprule  
    \multirow{2}{*}{\textbf{Method}}&  
    \multicolumn{2}{c}{\textbf{Flame Steak}}&\multicolumn{2}{c}{\textbf{Flame Salmon}}&\multicolumn{2}{c}{\textbf{Coffee Martini}}\cr  
    \cmidrule(lr){2-3}\cmidrule(lr){4-5}\cmidrule(lr){6-7}
    &\textbf{PSNR}$\uparrow$&\textbf{SSIM}$\uparrow$&\textbf{PSNR}$\uparrow$&\textbf{SSIM}$\uparrow$&\textbf{PSNR}$\uparrow$&\textbf{SSIM}$\uparrow$\cr  
    \midrule
    IN2N~\cite{haque2023instruct}+HexPlane~\cite{hexplane}&17.31&0.656&16.25&0.649&15.56&0.640\cr
    I4D-to-4D~\cite{mou2024instruct}&19.68&0.704&18.92&0.696&18.16&0.683\cr
    Ours&22.31&0.724&21.10&0.719&20.15&0.709\cr
    \bottomrule  
\end{tabular}}  
\end{table*}

\begin{table*}	
\centering  
% \fontsize{6.5}{8}\selectfont  
\caption{Per-Scene results of HyperNeRF's vrig datasets~\cite{park2021hypernerf} by different models.}  
\label{tab:hypernerf_comparison}  
\begin{tabular}{l|cc|cc|cc|cc}  
\toprule  
\multirow{2}{*}{\textbf{Method}}&  
\multicolumn{2}{c}{\textbf{3D Printer}}&\multicolumn{2}{c}{\textbf{Chicken}}&\multicolumn{2}{c}{\textbf{Broom}}&\multicolumn{2}{c}{\textbf{Banana}}\cr  
\cmidrule(lr){2-3}\cmidrule(lr){4-5}\cmidrule(lr){6-7}\cmidrule(lr){8-9}
&\textbf{PSNR}$\uparrow$&\textbf{MS-SSIM}$\uparrow$&\textbf{PSNR}$\uparrow$&\textbf{MS-SSIM}$\uparrow$&\textbf{PSNR}$\uparrow$&\textbf{MS-SSIM}$\uparrow$&\textbf{PSNR}$\uparrow$&\textbf{MS-SSIM}$\uparrow$\cr  
\midrule  
IN2N~\cite{haque2023instruct}+HexPlane~\cite{hexplane}&14.16&0.627&16.84&0.654&16.30&0.647&16.96&0.670\cr  
I4D-to-4D~\cite{mou2024instruct}&17.93&0.713&20.62&0.742&20.17&0.739&19.88&0.738\cr
PSF-4D (Ours)&20.16&0.753&23.83&0.815&19.62&0.748&22.31&0.808\cr
\bottomrule  
\end{tabular}  
\end{table*}

\begin{table*}[htb]
\centering
\caption{ \textbf{Ablation Study} on number of refinement steps, $L$. Although the longer refining phase produces slightly better results, the computational burden for performing these extra refining steps. Considering both performance and computation, we choose $L = 3$. }
% \vspace{-2mm}
\label{tab:refinement_comparison}
\scalebox{0.85}{\begin{tabular}{l|ccccc}
\toprule
\textbf{Refinement Steps, $L$} & \textbf{FID} $\downarrow$ & \textbf{CLIP Similarity} $\uparrow$ & \textbf{PSNR}$\uparrow$ & \textbf{SSIM}$\uparrow$ & \textbf{LPIPS}$\downarrow$ \\
\midrule
1 ($\omega_1 = 0.9$) & 21.23 & 0.3074 & 20.18 & 0.707 & 0.410 \\
2 ($\omega_2 = 0.75$)  & 22.15 & 0.3194 & 21.36 & 0.720 & 0.429 \\
3 ($\omega_3 = 0.6$) & 22.58 & 0.3241 & 22.17 & 0.726 & 0.436  \\
5 ($\omega_5 = 0.5$) & \textbf{22.81} & \textbf{0.3275} & \textbf{22.48} &\textbf{0.728} & \textbf{0.439}\\
\bottomrule
\end{tabular}}
% \vspace{-3mm}
\end{table*}

By leveraging this deformation-based approach, 4D-GS significantly reduces storage and memory overhead while maintaining rendering and training efficiency. The transformed 3D Gaussians are directly splatted onto the image plane to render dynamic scenes in real-time. For loss functions, we use L1 and TV loss. For the multi-resolution HexPlane module, the base resolution is set at 64, which is further upsampled by factors of 2 and 4. The initial learning rate is configured as $1.6 \times 10^{-3}$ and is reduced to $1.6 \times 10^{-4}$  by the end of training. The Gaussian deformation decoder is implemented as a compact multi-layer perceptron (MLP), with a learning rate starting at $1.6 \times 10^{-4}$ and decaying to $1.6 \times 10^{-5}$. Training is performed with a batch size of 2. For DyNeRF dataset, the training goes on for about 12,000 iterations for satisfactory rendering quality. For original model training, we need to initially keep more than 300K points through dense point-cloud reconstruction, which is later pruned to less than 100K points. 

\paragraph{4D Edited Model.} We first take a pre-trained IP2P model and convert it to a T2V model following the steps in TAV~\cite{wu2023tune}. TAV introduced a tailored spatio-temporal attention mechanism to capture continuous motion and an efficient one-shot tuning strategy. For training, we fine-tune the T2V model (with view-aware position encoding) on multi-view data.  During inference, we employ Denoising Diffusion Implicit Models (DDIM) inversion to provide structural guidance for sampling, lasting 30 steps. We use a classifier-free guidance of 7.5 for most scenes while going up to 9 for some scenes.  With our ANM noise model, we can achieve better motion smoothness in the generated videos. We also employ CNM noise model for spatial coherence across views. Combining ANM and CNM, we finally get the edited videos and re-train the 4D model on these videos. The training runs for 2500 iterations, with a batch size of 4. In our work, we use 30 text prompts to edit different scenes of all datasets. We then refine the edited model with view consistent refinement, which consists of total $L=3$ steps. In our work, four RTX A6000 GPUs were used to generate all our experiment results, allowing us to train four different models simultaneously with no distribution training.

% \begin{figure}[t]
%     \centering
%     \includegraphics[width=1.0\linewidth]{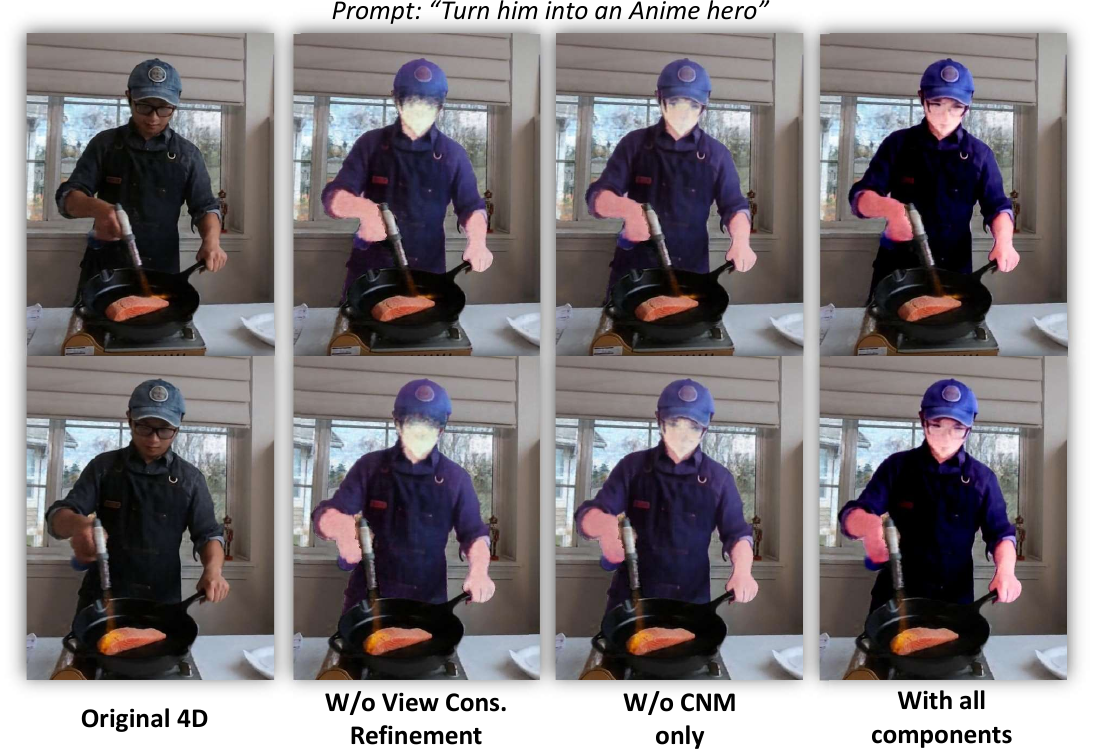}
%     \vspace{-2mm}
%     \caption{\footnotesize \textbf{Ablation on different components of our proposed method. } We show the impact of CNM and view consistent refinement in obtaining the desired editing effect. PSF-4D w/o view consistent refinement (VCR) indicates we edit the model only once ($L=0$), resulting in poor editing. Without CNM, the initial edited 4D model's quality drops significantly. However, quality improvement can be observed with iterative VCR. These results suggested that VCR plays the most important role in achieving the SOTA 4D editing performance.}
%     \vspace{-2mm}
%     \label{fig:main_ablation}
% \end{figure}

\begin{figure}[t]
    \centering
    \includegraphics[width=0.8\linewidth]{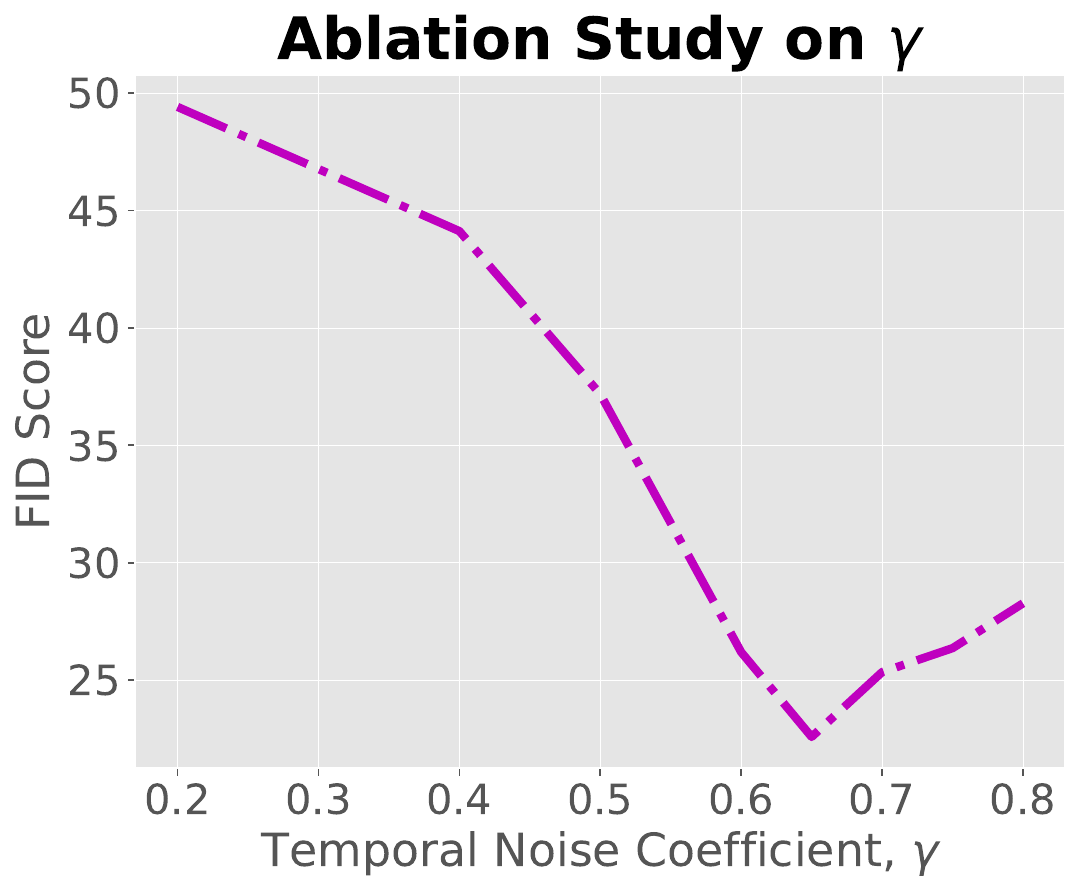}
    \caption{\textbf{Ablation Study on temporal noise coefficient, $\gamma$} in ANM noise model. The value of $\gamma$ determines how much weight T2V model puts on the previous window of frames while generating the current window of frames. The optimal value is $\gamma = 0.65$. Choosing a higher value puts a tighter constraint on the generation which eventually leads to suboptimal performance. We calculate the fidelity over all generated frames of DyNeRF datasets. A total of 8 distinct prompts are utilized for generating edits.}
    \label{fig:temporal_ablation}
\end{figure}

\begin{figure}[t]
    \centering
    \includegraphics[width=0.8\linewidth]{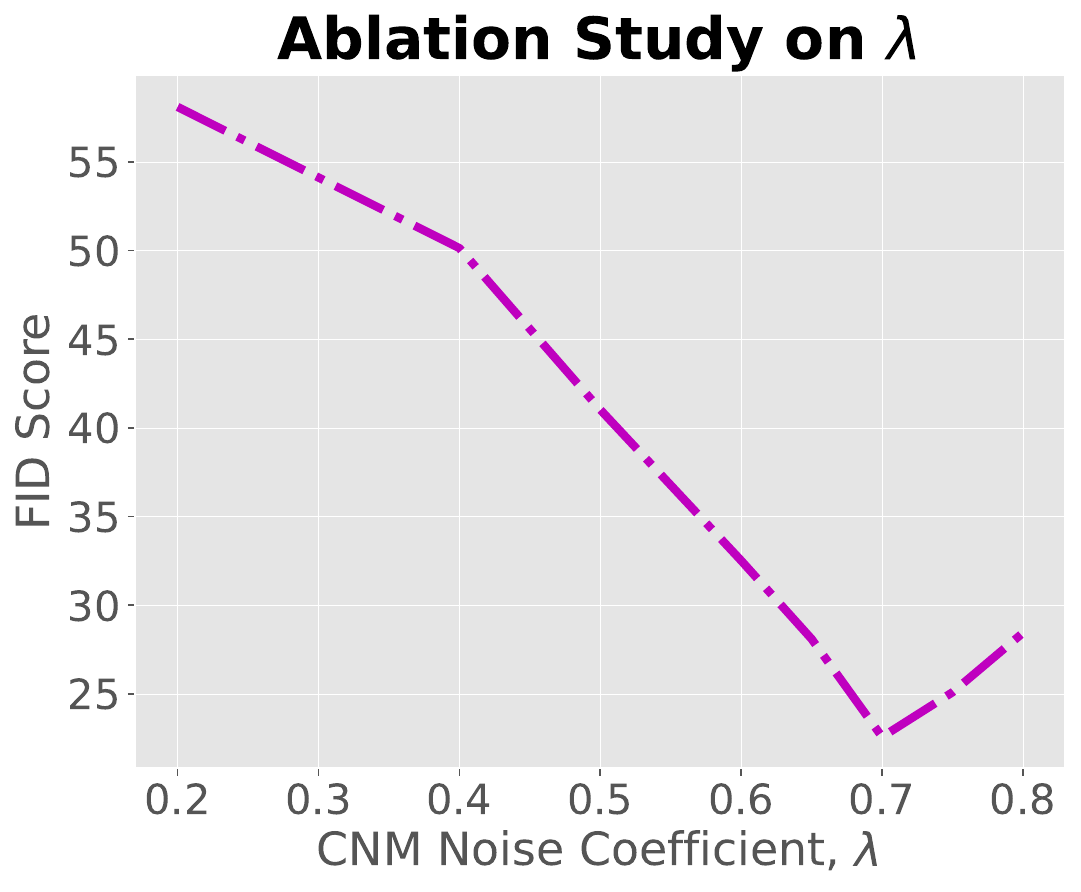}
    \caption{\textbf{Ablation Study on cross-view noise coefficient, $\lambda$} in CNM noise model. A lower value of $\lambda$ results in less consistent editing across different views due to reduced correlation between intermediate latents in T2V. Conversely, selecting a value greater than 0.7 makes it challenging to capture nuances in view-specific changes. This experiment is conducted using the Dy-NeRF dataset. }
    \label{fig:view_ablation}
\end{figure}

\begin{figure}[htb]
    \centering
    \includegraphics[width=0.8\linewidth]{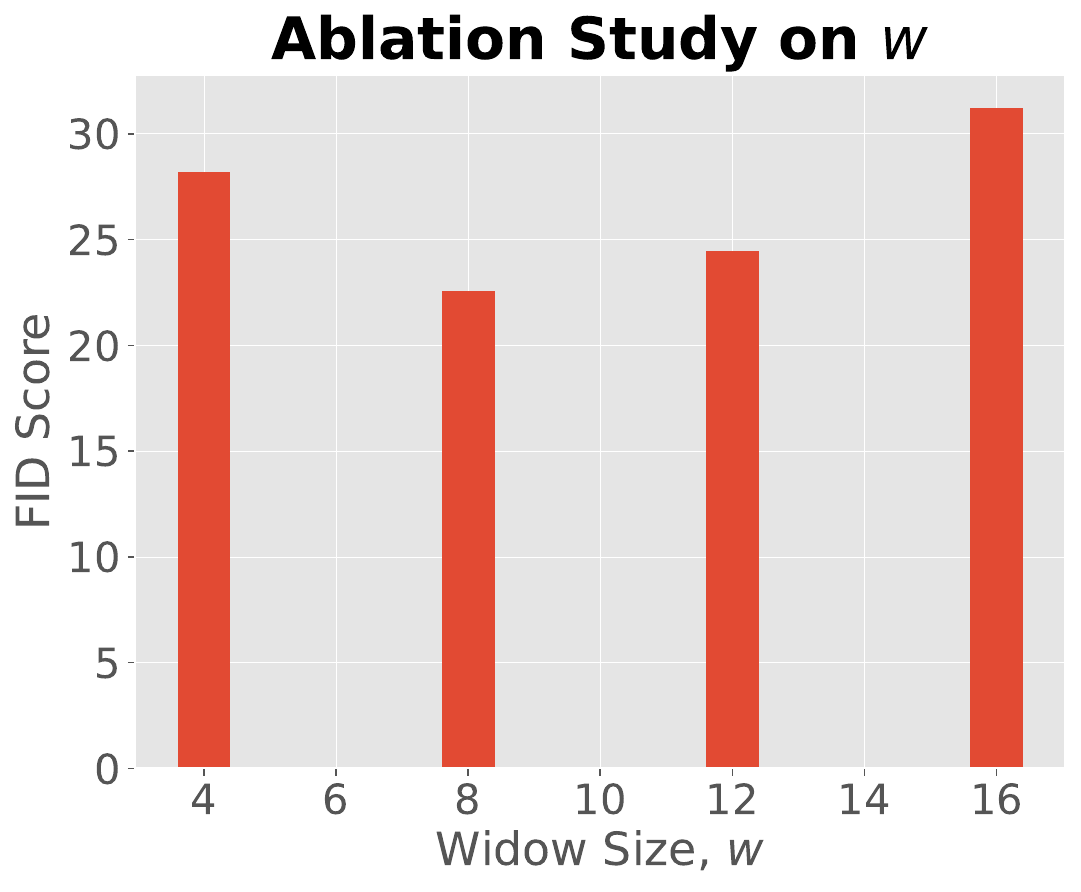}
    \caption{\textbf{Ablation Study on the video window size, $w$}. Here, we use $w = 8$ number of frames in each window. Given a fixed number of frames in a dataset, temporal consistency at later frames is hard to achieve if $w$ is small (the number of windows $n$ is low). Due to the current limitations of T2V models, intra-window consistency deteriorates once we increase the window size. We consider Dy-NeRF dataset for this.}
    \label{fig:window_ablation}
\end{figure}

\begin{figure*}[t]
    \centering
    \includegraphics[width =1\textwidth]{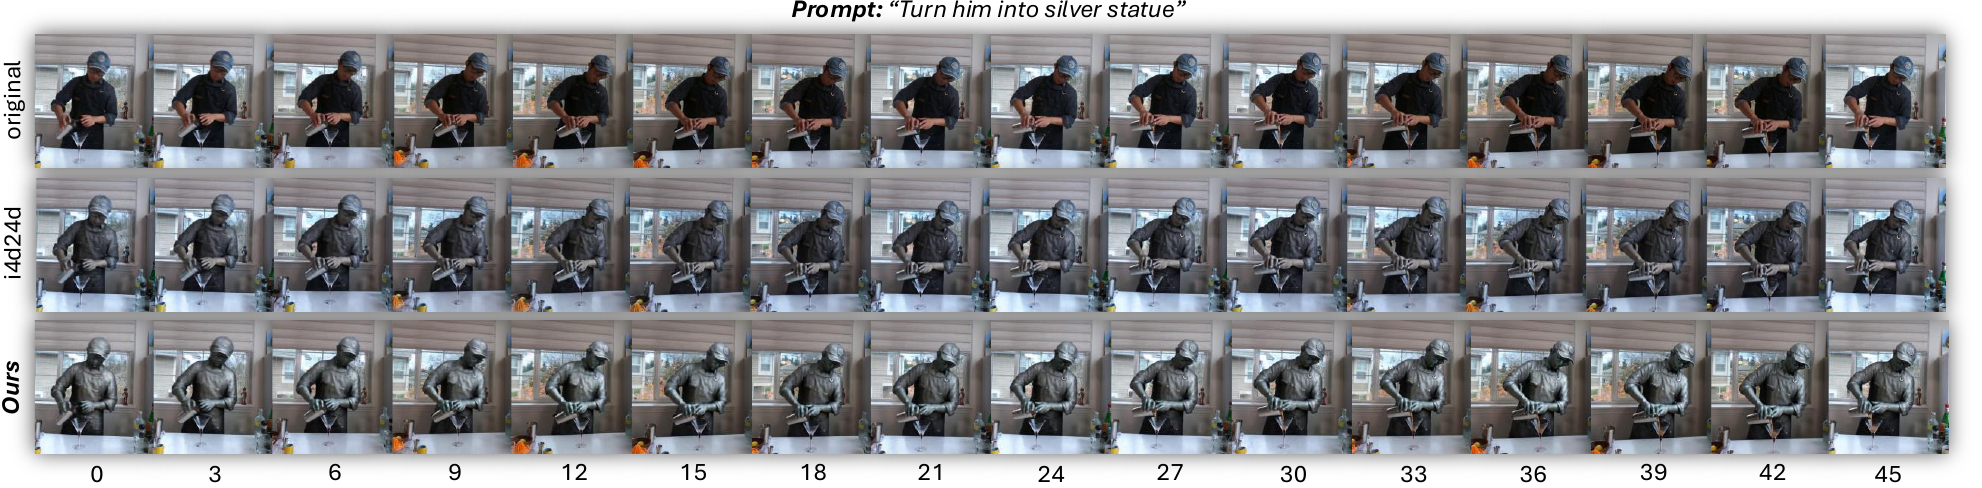}
    \caption{\textbf{Frame-by-frame Video Comparison} at selected intervals (0, 6, …, 45) between I4D-to-4D and SPF4D (ours).}
    \label{fig:rebuttal_fig}
\end{figure*}

\subsection{Evaluation Metrics}\label{sec:eval_metrics}
In addition to FID and CLIP Similarity score, the evaluation of visual quality is conducted using LPIPS~\cite{zhang2018unreasonable}, Structural Similarity Index (SSIM)~\cite{wang2004image}, Multi-scale Structural Similarity Index (MS-SSIM)~\cite{wang2003multiscale}, and PSNR metrics. However, due to the reconstruction of dynamic scenes from a single moving camera, slight deviations in geometry or appearance may occur, introducing ambiguities. These discrepancies often cause standard quantitative metrics to fail in capturing perceptual quality accurately. For instance, PSNR is highly sensitive to minor shifts, often favoring blurred outputs over sharp ones, while MS-SSIM may overlook artifacts that are noticeable to human observers. Among these metrics, LPIPS is identified as the most reliable indicator of perceptual quality. 

\subsection{Baseline Implementations}\label{sec:baseline_implement}
We consider 2 other baselines for comparison. Although Control4D~\cite{shao2023control4d} is a similar 4D editing work, we could not report the comparisons here as no implementation was available. 
For I4D-to-4D, we follow the implementation here\footnote{\href{I4D-to-4D}{https://github.com/Friedrich-M/Instruct-4D-to-4D/}} where the NeRF-based 4D editing was performed which usually takes a higher number of iterations (around 100K). We follow the implementations here~\footnote{\href{InstructNeRF2NeRF}{https://github.com/ayaanzhaque/instruct-nerf2nerf}} for InstructNeRF2NeRF and this codebase~\footnote{\href{HexPlance}{https://github.com/Caoang327/HexPlane}} for Hexplane. We iterative update all the frames of a scene sequentially, without employing any spatiotemporal attention of T2V.   

\section{Quantitative Results}\label{sec:quantitative_results}
In Table~\ref{tab:comparison_all_datasets}, we compare the performance of PSF-4D with other methods. Due to the proposed noise model design and iterative refinement, PSF-4D achieves superior results in all datasets by a significant margin. These improvements indicate that controlled noise in the diffusion model enforces generation with greater temporal and view consistency. Table~\ref{tab:dynerf_comparison}-\ref{tab:hypernerf_comparison} shows per-scene statistics for Dy-NeRF and HyperNeRF datasets. It can be observed that some scenes are relatively more complex than others. For the HyperNeRF dataset, we consider the MS-SSIM metric as suggested in the original work.   

\subsection{Local Editing}\label{sec:local_editing}
In addition to SAM, we modify the "target editing prompt", $C_T$ with GPT-4~\cite{achiam2023gpt} and LlaVA~\cite{lin2023video}. For example, if we feed the "Coffee Martini" video from Dy-NeRF dataset to LLaVA, the description looks like this, \( C_D \): \emph{"The video features a person standing behind a white countertop in what appears to be a home bar setup. The individual is wearing a dark apron and a cap, suggesting they are preparing a drink. On the countertop, there is an array of items including a juicer with orange juice, a cocktail shaker, a glass filled with ice, and several bottles of alcohol. The background shows a window with blinds partially drawn, allowing natural light into the room. The person is seen pouring liquid from the cocktail shaker into the glass, indicating the process of making a cocktail."} 

Consider the target prompt to be, $C_T$: "Turn him into an Anime Hero". Now we feed this description and target caption to GPT-4, we get the final editing prompt, \( C_S \): \emph{"Transform the person into an anime hero with spiky hair, a vibrant outfit, and a glowing aura, keeping the home bar setup and cocktail-making intact."} \( C_S \) has been used to edit the final 4D model.

\section{Ablation Study}\label{sec:ablation_study}
We provide the ablation on different hyperparameters below.

\subsection{Ablation on $\gamma$}
Figure~\ref{fig:temporal_ablation} shows the FID scores for different values of $\gamma$. As shown in the main paper, $\gamma$ determines the nature of noise initialization in the T2V model and helps us obtain better temporal consistency. For all these ablations, we consider the Dy-NeRF dataset.
\subsection{Ablation on $\lambda$}
In Figure~\ref{fig:view_ablation}, we present the ablation on $\lambda$. If we choose a smaller value, the model struggles to preserve the commonalities between views. 
\subsection{Ablation on window size, $w$}
Figure~\ref{fig:window_ablation} illustrates the performance variation when we change the window size of a video. 
\subsection{Ablation on refinement steps, $L$}
Table~\ref{tab:refinement_comparison} shows the impact of the view-consistent refinement process over time. If we refine the edited 4D model for longer, the computation burden will be significant as it takes 25-30 minutes for each refinement step. We also linearly reduce the value of $\omega_l$ as the refinement progresses.

\section{Comparison With I4D-to-4D}\label{sec:comparison}
We provide frame-by-frame comparison with I4D-to-4D in Figure~\ref{fig:rebuttal_fig}. We also provide the video comparison in the Supplementary.

% % 
% Having the supplementary compiled together with the main paper means that:
% % 
% \begin{itemize}
% \item The supplementary can back-reference sections of the main paper, for example, we can refer to \cref{sec:intro};
% \item The main paper can forward reference sub-sections within the supplementary explicitly (e.g. referring to a particular experiment); 
% \item When submitted to arXiv, the supplementary will already included at the end of the paper.
% \end{itemize}
% % 

% To split the supplementary pages from the main paper, you can use \href{https://support.apple.com/en-ca/guide/preview/prvw11793/mac#:~:text=Delete%20a%20page%20from%20a,or%20choose%20Edit%20%3E%20Delete).}{Preview (on macOS)}, \href{https://www.adobe.com/acrobat/how-to/delete-pages-from-pdf.html#:~:text=Choose%20%E2%80%9CTools%E2%80%9D%20%3E%20%E2%80%9COrganize,or%20pages%20from%20the%20file.}{Adobe Acrobat} (on all OSs), as well as \href{https://superuser.com/questions/517986/is-it-possible-to-delete-some-pages-of-a-pdf-document}{command line tools}.
